# Supplementary material for: Fractionalization paves the way to local projector embeddings of quantum many-body scars
Source: arXiv:2305.00827 source file (2023-05-01)
Supplement: Supplementary file 1 [file appendix.tex]

\section{Another proof of the scar states in the spin-1 XY model}\label{app:another proof XY}
Here we provide another proof of the scar states $\ket*{\mc{S}_n^{\mr{XY}}}$ in the spin-$1$ XY model. This proof covers the case $N=4k+2$ for $k\in\mb{N}$, but requires an involved calculation.

We define another unitary twist transformation:
\begin{equation}
    U'_\pi\coloneqq\exp\left[i\pi\sum_{j\in\Lambda}jP_j^+\right],
\end{equation}
where $P_j^\sigma\coloneqq\dyad*{\sigma}_j$ for $\sigma=\pm, 0$. This operator is compatible with the boundary condition since $e^{i\pi NP_j^+}=1$ for $N$ even. 

This operator yields the same conjugated creation operator $U'_\pi Q_{\mr{XY}}^+U'^\dag_\pi=J^+_{\mr{XY}}$. 

We next explicitly calculate the conjugated XY-term and find
\begin{equation}
    \begin{split}
        &U'_\pi\left(S_i^xS_{i+1}^x+S_i^yS_{i+1}^y\right)U'^\dag_{\pi}P_i^{\mc{W}}=(-1)^i\ket{0,0}\left(\bra{+,-}-\bra{-,+}\right)_{i,i+1}P_i^{\mc{W}}.%\\&
        %+(-1)^i\left(\ket{+,-}-\ket{-,+}\right)\bra{0,0}_{i,i+1}\\
        %&-\dyad{+,0}{0,+}_{i,i+1}-\dyad{0,+}{+,0}_{i,i+1}\\
        %&+\dyad{-,0}{0,-}_{i,i+1}+\dyad{0,-}{-,0}_{i,i+1}.
    \end{split}
\end{equation}
The conjugated scar states are again characterized by local projectors $\wtil{P}^{\mr{as}}_{i,i+1}P^{\mc{W}}_i$ and $1-P^{\mc{W}}_i$, and fully symmetric within $\mc{W}$.
\section{A detailed proof of $\ket*{\mc{B}_n}$}\label{sec:app XY}
In this appendix, we prove  the states $\ket*{\mc{B}_n}$ defined in Eq.~\eqref{eq:bimagnon spin-1/2} to be exact eigenstates of $H_{\mr{XY}}$, provided the single ion anisotropy vanishes, $D=0$. Like the AKLT model, as the mapping from fractionalized spins to $S=1$ spins $\msf{A}_{\mr{XY}}:\mb{C}^{2\otimes2\otimes N}\rightarrow\mb{C}^{3\otimes N}$ is not injective, there is no unique choice for the operator $O_{\mr{frac}}$ on $\mb{C}^{2\otimes2\otimes N}$ that satisfy $O\msf{A}_{\mr{XY}}=\msf{A}_{\mr{XY}}O_{\mr{frac}}$ for a given spin-$1$ operator $O$ on $\mb{C}^{3\otimes N}$. For example, both $\msf{A}_{\mr{XY}}\dyad*{\downarrow\uparrow}{\uparrow\uparrow}_{(i,\mr{L}),(i+1,\mr{R})}$ and $\msf{A}_{\mr{XY}}\dyad*{\uparrow\downarrow}{\uparrow\uparrow}_{(i,\mr{L}),(i,\mr{R})}$ yield $\dyad{0}{+}_i\msf{A}_{\mr{XY}}$. Therefore, we have some  freedom in choosing $H_{\mr{XY}}^{\mr{frac}}$ such that $H_{\mr{XY}}\msf{A}_{\mr{XY}}=\msf{A}_{\mr{XY}}H_{\mr{XY}}^{\mr{frac}}$. 

Here we will show that one can choose a suitable operator $H_{\mr{XY}}^{\mr{frac}}$, such  that $\msf{A}_{\mr{XY}}H_{\mr{XY}}^{\mr{frac}}=H_{\mr{XY}}\msf{A}_{\mr{XY}}$ and $\ket*{\mc{B}_n^{\mr{frac}}}$ defined in Eq.~\eqref{eq:bimagnon spin-1/2} is an eigenstate of $H_{\mr{XY}}^{\mr{frac}}$%$\ket*{\mc{B}_n^{\mr{frac}}}=E_n\ket*{\mc{B}_n^{\mr{frac}}}$ holds (for $D=0$), it immediately follows that %$\ket*{\mc{B}_n}$ is  a scar state. With this setting, we show that $\ket*{\mc{B}_n}$ is 
%an eigenstate of $H_{\mr{XY}}$
, and that one can define an operator $T_{\mr{XY},i}^{\mr{frac}}$ such that $\sum_{i\in\Lambda}S_i^xS_{i+1}^x+S_i^yS_{i+1}^y\msf{A}_{\mr{XY}}=\msf{A}_{\mr{XY}}\sum_{i\in\Lambda}T_{\mr{XY},i}^{\mr{frac}}$ holds and $T_{\mr{XY},i}^{\mr{frac}}$ annihilates the bimagnon states. 
\begin{proof} We first define the  map $\wtil{M}_i:\mb{C}^2\rightarrow\mb{C}^{2\otimes2}$ as
\begin{equation}
    \wtil{M}_i\coloneqq\ket*{\uparrow\uparrow}_{(i,\mr{R}),(i+1,\mr{L})}\bra*{\uparrow}_i+\ket*{\downarrow\downarrow}_{(i,\mr{R}),(i+1,\mr{L})}\bra*{\downarrow}_i,
\end{equation}
%which is 'shifted by one fractional spin' as compared to the standard embedding.
and $\wtil{\msf{M}}\coloneqq\bigotimes_{i\in\Lambda}\wtil{M}_i$. We consider the subspace $\mc{W}\subset\mb{C}^{2\otimes2\otimes N}$ as 
\begin{equation}
    \mc{W}\coloneqq\left\{\wtil{\msf{M}}\ket*{\psi}\big|\ket*{\psi}\in\mb{C}^{2\otimes N}\right\}.
\end{equation}
In what follows, we write $\ket{\bm{\sigma}}_{i^*}\coloneqq \ket{\sigma\sigma}_{i^*}= \wtil{M}_i\ket*{\sigma}_i$ with $i^*\coloneqq((i,\mr{R}),(i+1,\mr{L}))$, denoting the pair of equal fractional spins with a bold letter. It is easy to see that the fractional scar states defined in Eq.~\eqref{eq:bimagnon spin-1/2} belong to $\mc{W}$, $\ket*{\mc{B}^{\mr{frac}}_n}\in\mc{W}$. We call $P_{i^*}^{\mc{W}}=\dyad*{\bm{\uparrow}}+\dyad*{\bm{\downarrow}}_{i^*}$ the local projector onto $\mc{W}$. %Within the subspace, the ladder operators in Eq.~\eqref{eq:ladder mod.} are simplified further. For example, one can check
%\begin{equation}\label{eq:ladder mod2.}\begin{split}
    %S_i^+\msf{A}P^\uparrow_{(i-1,\mr{R})}P_{\mc{W},i^*}&=\sqrt{2}\msf{A}P^{\bm{\uparrow}}_{(i-1)^*}\sigma^+_{(i,\mr{R})}P_{\mc{W},i^*}\\
    %S_i^+\msf{A}P^\downarrow_{(i-1,\mr{R})}P_{\mc{W},i^*}&\sqrt{2}=\msf{A}\dyad*{\downarrow\uparrow}{\downarrow\downarrow}_{(i-1,\mr{R}),(i,\mr{L})}P_{\mc{W},i^*}\\
    %S_i^+\msf{A}P^\uparrow_{(i+1,\mr{L})}P_{\mc{W},i^*}&=\sqrt{2}\msf{A}\sigma^+_{(i,\mr{L})}P^{\bm{\uparrow}}_{i^*}P_{\mc{W},i^*}\\
    %S_i^+\msf{A}P^\downarrow_{(i+1,\mr{L})}P_{\mc{W},i^*}&=\sqrt{2}\msf{A}\dyad*{\uparrow\downarrow}{\downarrow\downarrow}_{(i,\mr{R}),(i+1,\mr{L})}P_{\mc{W},i^*},
   %\end{split}
%\end{equation}
%where $P_{i^*}^{\bm{\sigma}}\coloneqq\dyad*{\bm{\sigma}}_{i^*}$. Similar relations hold for $S^-_i$ as well.
We shall then find an operator $T^{+,-}_{i,i+1}$ satisfying $\msf{A}_{\mr{XY}}T_{i,i+1}^{+,-}=(S_i^+S_{i+1}^-/2)\msf{A}_{\mr{XY}}$. Using the freedom in choosing proper operators in the $S=1/2$ space mentioned above, we obtain
\begin{equation}\label{eq:T+-}
    \begin{split}
        \dyad*{+,0}{0,+}_{i,i+1}\msf{A}_{\mr{XY}}P_{i^*}^{\mc{W}}&=\msf{A}_{\mr{XY}}\dyad*{\uparrow\uparrow,\downarrow\uparrow}{\downarrow\uparrow,\uparrow\uparrow}_{i,i+1}P_{i^*}^{\mc{W}}\\
        \dyad*{+,-}{0,0}_{i,i+1}\msf{A}_{\mr{XY}}P_{i^*}^{\mc{W}}&=\msf{A}_{\mr{XY}}\left(\dyad*{\uparrow\uparrow,\downarrow\downarrow}{\uparrow\downarrow,\downarrow\uparrow}+\dyad*{\uparrow\uparrow,\downarrow\downarrow}{\downarrow\uparrow,\uparrow\downarrow}\right)_{i,i+1}P_{i^*}^{\mc{W}}\\
        \dyad*{0,0}{+,-}_{i,i+1}\msf{A}_{\mr{XY}}P_{i^*}^{\mc{W}}&=0\\
        \dyad*{0,-}{-,0}_{i,i+1}\msf{A}_{\mr{XY}}P_{i^*}^{\mc{W}}&=\msf{A}_{\mr{XY}}\dyad*{\downarrow\uparrow,\downarrow\downarrow}{\downarrow\downarrow,\downarrow\uparrow}_{i,i+1}P_{i^*}^{\mc{W}},
    \end{split}
\end{equation}
where $\ket*{\sigma\sigma'}_i\equiv\ket*{\sigma\sigma'}_{(i,\mr{L}),(i,\mr{R})}$. Eq.~\eqref{eq:T+-} implies that $T_{i,i+1}^{+,-}$ is written as
\begin{equation}\begin{split}\label{eq:T+-P}
    T_{i,i+1}^{+,-}&=\left(\dyad*{\uparrow\downarrow,\downarrow\uparrow}{\bm{\downarrow},\bm{\uparrow}}_{i^*,(i+1)^*}+\dyad*{\downarrow\uparrow,\uparrow\downarrow}{\bm{\downarrow},\bm{\uparrow}}_{(i-1)^*,i^*}\right)P^{\mc{W}}_{(i-1)^*}P^{\mc{W}}_{i^*}P_{(i+1)^*}^{\mc{W}}\\&+T_{i,i+1}^{+,-}\left(1-P^{\mc{W}}_{(i-1)^*}P^{\mc{W}}_{i^*}P^{\mc{W}}_{(i+1)^*}\right),
    \end{split}
\end{equation}
where $\ket*{\sigma\sigma'}_{i^*}\equiv\ket*{\sigma\sigma'}_{(i,\mr{R}),(i+1,\mr{L})}$. Similarly, we can find the operator $T_{i,i+1}^{-,+}$ satisfying $\msf{A}_{\mr{XY}}T_{i,i+1}^{-,+}=(S_i^-S_{i+1}^+)/2\msf{A}_{\mr{XY}}$,
\begin{equation}\label{eq:T-+P}
    \begin{split}
        T_{i,i+1}^{-,+}&=\left(\dyad*{\downarrow\uparrow,\uparrow\downarrow}{\bm{\uparrow},\bm{\downarrow}}_{i^*,(i+1)^*}+\dyad*{\uparrow\downarrow,\downarrow\uparrow}{\bm{\uparrow},\bm{\downarrow}}_{(i-1)^*,i^*}\right)P_{(i-1)^*}^{\mc{W}}P^{\mc{W}}_{i^*}P_{(i+1)^*}^{\mc{W}}\\&+T_{i,i+1}^{-,+}\left(1-P^{\mc{W}}_{(i-1)^*}P^{\mc{W}}_{i^*}P^{\mc{W}}_{(i+1)^*}\right).
    \end{split}
\end{equation}

Combining Eq.~\eqref{eq:T+-P} and Eq.~\eqref{eq:T-+P}, we can decompose $\sum_{i\in\Lambda}S_i^xS_{i+1}^x+S_i^yS_{i+1}^y$ as a sum of local annihilators in the $S=1/2$ space,
\begin{equation}
    \begin{split}
        &\left(\sum_{i\in\Lambda}S_i^xS_{i+1}^x+S_i^yS_{i+1}^y\right)\msf{A}_{\mr{XY}}\\&=\msf{A}_{\mr{XY}}\sum_{i\in\Lambda}\left(\ket*{\uparrow\downarrow,\downarrow\uparrow}+\ket*{\downarrow\uparrow,\uparrow\downarrow}\right)\left(\bra*{\bm{\uparrow},\bm{\downarrow}}+\bra*{\bm{\downarrow},\bm{\uparrow}}\right)_{i^*,(i+1)^*}P^{\mc{W}}_{i^*}P_{(i+1)^*}^{\mc{W}}\\
        &+\msf{A}_{\mr{XY}}\sum_{i\in\Lambda}h_i\left(1-P^{\mc{W}}_{i^*}P_{(i+1)^*}^{\mc{W}}\right)\\
        &\equiv\msf{A}_{\mr{XY}}\left(\sum_{i\in\Lambda}T_{\mr{XY},i}^{\mr{frac}}\left(P_{i^*}^{\mc{W}}P_{(i+1)^*}^{\mc{W}}+\left(1-P^{\mc{W}}_{i^*}P_{(i+1)^*}^{\mc{W}}\right)\right)\right),
    \end{split}
\end{equation}
where $h_i$ is a some local operator. The third line trivially annihilates $\ket*{\mc{B}_n^{\mr{frac}}}$ locally since $\ket*{\mc{B}_n^{\mr{frac}}}\in\mc{W}$. Thus, it is sufficient to show that $T_{\mr{XY},i}^{\mr{frac}}$ also annihilates $\ket*{\mc{B}_n^{\mr{frac}}}$ locally. To do so, we consider the following unitary operator on $\mb{C}^{2\otimes2\otimes N}$ that rotates blocks of two fractional spins by a linearly increasing angle around the $z$-axis:
\begin{equation}
    U_\pi\coloneqq\exp\left[i\pi\sum_{j\in\Lambda}jP^{\bm{\uparrow}}_{j^*}\right],
\end{equation}
which leaves $\mc{W}$ invariant. This operator is compatible with the boundary condition since $e^{i\pi NP_{j^*}^{\bm{\uparrow}}}=1$ for $N$ even. The twisted scar states $U_\pi\ket*{\mc{B}^{\mr{frac}}_n}$ are fully symmetric with respect to permutations of block spins $\ket{\bm{\sigma}}_{i^*}$. This follows from $U_\pi Q^+_{\mr{bm}}U_\pi^\dag=\sum_{i\in\Lambda}\sigma^+_{(i,\mr{R})}\sigma^+_{(i+1,\mr{L})}=\sum_{i\in\Lambda}\dyad*{\bm{\uparrow}}{\bm{\downarrow}}_{i^*}$ and $U_\pi\ket*{\mc{B}_0^{\mr{frac}}}=\ket*{\mc{B}_0^{\mr{frac}}}=\bigotimes_{i\in\Lambda}\ket*{\bm{\downarrow}}_{i^*}$.

It is straightforward to check that $T_{\mr{XY},i}^{\mr{frac},U}\coloneqq U_\pi T_{\mr{XY},i}^{\mr{frac}}U_\pi^\dag$ is unaltered when the projectors $P_{i^*,(i+1)^*}^{\mr{as}}\equiv\wtil{\msf{M}}P^{\mr{as}}_{i,i+1}\wtil{\msf{M}}$ is acted upon it from the right. Thus, it should annihilate $U_\pi\ket*{\mc{B}_n^{\mr{frac}}}$. % $T_{\mr{XY},i}^{\mr{frac},(U)}\coloneqq U_\pi T_{\mr{XY},i}^{\mr{frac}}U^\dag_\pi$ is unaltered when multiplied from the right by a factor $P_{\mr{asym},i^*}P_{\mc{W},i^*}+(1-P_{\mc{W},i^*})$ where $P_{\mr{asym},i^*}=(1-sw_{(i-1)^*,i^*})/2$ projects onto states antisymmetric with respect to a swap of block spins at bonds $(i-1)^*\leftrightarrow i^*$. Thus, it annihilates $U_\pi\ket*{\mc{B}_n^{\mr{frac}}}$.

Finally we consider the remaining Zeeman term. %Although we have freedom in choosing spin-$1/2$ operator $O_{\mr{frac}}$ such that 
A natural way to lift $S_i^z$ to the fractional spin space uses the identity
%$\msf{A}O_{\mr{frac}}=O\msf{A}$ for a given $O$ in general, $S^z$ induces a spin-$1/2$ operator quite naturally:
    \begin{equation}
        S_i^z\msf{A}_{\mr{XY}}=\msf{A}_{\mr{XY}}\left(\dyad*{\uparrow\uparrow}-\dyad*{\downarrow\downarrow}\right)_{(i,\mr{L}),(i,\mr{R})}=\msf{A}_{\mr{XY}}\frac{1}{2}\left(\sigma_{(i,\mr{L})}^z+\sigma_{(i,\mr{R})}^z\right)
    \end{equation}
such that the Zeeman term can simply be written as $\sum_{i\in\Lambda}S_i^z\msf{A}_{\mr{XY}}=\frac{1}{2}\msf{A}\sum_{\alpha\in\Lambda^{\mr{frac}}}\sigma_\alpha^z$. From the form of $\ket*{\mc{B}^{\mr{frac}}_n}$ it is then immediately clear that it is an eigenstate of the Zeeman term.
\end{proof}
%WHAT IS MISSING HERE:
%Indicate how one gets to the scar states of the original model.
%In the beginning you say we had a freedom to choose Hfrac, but nowhere you indicate where you used this freedom.

%Most importantly: Write the (lifted) Hamiltonian in a fashion that fits with our general shape.
%As far as I understand you say that Hfrac has genuine scar states in the unconstrained fractionalized Hilbert space. 

%Discuss explicitly whether the scar states respect the symmetrization constraint (between iL and iR), and if not, how it comes that scar states of H frac translate to scar states of H.
In summary, we showed that only in the fractional Hilbert space, the model is expressed as 
\begin{equation}
    \begin{split}
        H_{\mr{XY}}\msf{A}_{\mr{XY}}&=\msf{A}_{\mr{XY}}H^{\mr{frac}}_{\mr{XY}}\\
        H^{\mr{frac}}_{\mr{XY}}&=\frac{1}{2}\sum_{i\in\Lambda}\left(\sigma^z_{(i,\mr{L})}+\sigma^z_{(i,\mr{R})}\right)+\sum_{i\in\Lambda}T_{\mr{XY},i}^{\mr{frac}}\left(P^{\msf{M}}_i P_{i^*}^{\mc{W}}P_{(i+1)^*}^{\mc{W}}+\left(1-P_{i^*}^{\mc{W}}P_{(i+1)^*}^{\mc{W}}\right)\right),
    \end{split}
\end{equation}
where $P_i^{\msf{M}}\coloneqq U_\pi^\dag P^{\mr{as}}_{i^*,(i+1)^*}U_\pi$.
%a lift of the spin-$1/2$ model Eq.~\eqref{eq:toy model} after the twist unitary transformation, and that the fractionalized scar states $\ket*{\mc{B}_n^{\mr{frac}}}$ corresponds to the maximal spin states which are fully symmetric with respect to a site swap.
\section{Another proof of the scar states in the AKLT model}\label{app:another AKLT}
Here we shall prove that the scar states $\ket*{\mc{S}_n^{\mr{AKLT}}}$ are exact eigenstates of the AKLT model even when $N=4k+2$ for $k\in\mb{N}$. To do so, we show the following Lemma:
\begin{lemma}\label{lemma:AKLT}
$\ket*{\mc{S}_n^{\mr{frac}}}$ is expressed as
\begin{equation}\label{eq:lemma AKLT}\begin{split}
    \ket*{\mc{S}_n^{\mr{frac}}}&=\sum_{\bm{\sigma}\bm{\sigma'}}\ket*{\bm{\sigma\downarrow\sigma'}}_{(i-1)^*,i^*,(i+1)^*}\otimes\ket*{\Xi^0_{\sigma\sigma'}}+\left(\ket{\bm{\uparrow\uparrow\downarrow}}-\ket*{\bm{\downarrow\uparrow\uparrow}}\right)_{(i-1)^*,i^*,(i+1)^*}\otimes\ket*{\Xi^1}\\
    &+\ket*{\bm{\uparrow\uparrow\uparrow}}_{(i-1)^*,i^*,(i+1)^*}\otimes\ket*{\Xi^2},
    \end{split}
\end{equation}
where $\ket*{\Xi^i} (i=0,1,2)$ is an unnormalized state defined on all bonds expect $(i-1)^*, i^*,$ and $(i+1)^*$.
\end{lemma}
This statement immediately implies that $T_{i,i+1}^{\mr{frac}}\ket*{\mc{S}_n^{\mr{frac}}}=0$ from Eq.~\eqref{eq:AKLT SM form}. It also indicates $T_{i,i+1}^{\mr{frac}}=T_{i,i+1}^{\mr{frac}}(P^{\mr{sym}}_{i^*}P_{i^*}^{\bm{\uparrow}}P^{\mc{W}}_i+(1-P^{\mc{W}}_i))$ where $P^{\mr{sym}}_{i^*}=(1+sw_{(i-1)^*,(i+1)^*})/2$ projects onto block spin states symmetric with respect to a bond swap $(i-1)^*\leftrightarrow(i+1)^*$. Thus, as in Sec.~\ref{sec:AKLT}, the Hamiltonian in the fractional spin-$1/2$ space is expressed as a sum of the Zeeman term (corresponding to $H_{\mr{spec}}$) and local annihilators $T_{i,i+1}^{\mr{frac}}$ (corresponding to $H_{\mr{ann}}$).
\begin{proof}[Proof of Lemma.~\ref{lemma:AKLT}]
We show this statement by induction. When $n=0$, it is trivial since $\ket*{\mc{S}_0^{\mr{frac}}}=\bigotimes_{i\in\Lambda}\ket*{\bm{\downarrow}}_{i^*}$. Suppose if Eq.~\eqref{eq:lemma AKLT} is true for $n=k$, we find
\begin{equation}
    \begin{split}
        Q_{\mr{frac}}^+\ket*{\mc{S}_n^{\mr{frac}}}&=\sum_{\bm{\sigma\sigma'}}\ket*{\bm{\sigma\downarrow\sigma'}}_{(i-1)^*,i^*,(i+1)^*}\otimes\ket*{\wtil{\Xi}^0_{\sigma\sigma'}}+\left(\ket*{\bm{\uparrow\uparrow\downarrow}}-\ket*{\bm{\downarrow\uparrow\uparrow}}\right)_{(i-1)^*,i^*,(i+1)^*}\otimes\ket*{\wtil{\Xi}^1}\\&+\ket*{\bm{\uparrow\uparrow\uparrow}}_{(i-1)^*,i^*,(i+1)^*}\otimes\ket*{\wtil{\Xi}^2},
    \end{split}
\end{equation}
where
\begin{equation}
    \begin{split}
        \ket*{\wtil{\Xi}^0_{\sigma\sigma'}}&=\wtil{Q}_{\mr{frac}}^+\ket*{\Xi^0_{\sigma\sigma'}}\\
        \ket*{\wtil{\Xi}^1}&=(-1)^{i-1}\ket*{\Xi^0_{\downarrow\downarrow}}+\wtil{Q}_{\mr{frac}}^+\ket*{\Xi^1}\\
        \ket*{\wtil{\Xi}^2}&=(-1)^{i-1}\ket*{\Xi^0_{\downarrow\uparrow}}+(-1)^i\ket*{\Xi^0_{\uparrow\downarrow}}-(-1)^{i+1}\left(\dyad*{\bm{\uparrow}}{\bm{\downarrow}}_{(i-2)^*}+\dyad*{\bm{\uparrow}}{\bm{\downarrow}}_{(i+2)^*}\right)\ket*{\Xi^1}+\wtil{Q}_{\mr{frac}}^+\ket*{\Xi^2},
    \end{split}
\end{equation}
with $\wtil{Q}_{\mr{frac}}^+\coloneqq\sum_{j\in\Lambda\setminus\{i-2,i-1,i,i+1\}}(-1)^j\dyad*{\bm{\uparrow\uparrow}}{\bm{\downarrow\downarrow}}_{j^*,(j+1)^*}$. Thus, Eq.~\eqref{eq:lemma AKLT} holds true for $n=k+1$.
\end{proof}

\section{Proof of scar states in the spin-S AKLT model}\label{sec:app AKLT}
Here we show that the states $\ket*{\mc{S}^S_n}$ defined in Eq.~\eqref{eq:scar S-AKLT} are exact eigenstates of $H_{\mr{AKLT}}^S$. Note that there is a natural choice to lift an operator $O$ on $\mb{C}^{(2S+1)\otimes N}$ to an operator $O_{\mr{frac}}$ on $\mb{C}^{2\otimes 2S\otimes N}$ (the unconstrained fractionalized Hilbert space), such that $\wtil{\msf{A}}_{\mr{vb}}O_{\mr{frac}}=O\wtil{\msf{A}}_{\mr{vb}}$. Indeed, the identity
\begin{equation}\label{eq:extended identity}
    f(\{\bm{S}_i\}_{i\in\Lambda})\wtil{\msf{A}}_{\mr{vb}}=\wtil{\msf{A}}_{\mr{vb}}f\left(\left\{\sum_{l\in\lambda}\bm{S}_{(i,l)}\right\}_{i\in\Lambda}\right)
\end{equation}
suggests that one construct $O_{\mr{frac}}$ simply by writing $O$ as a polynomial in spin operators and  replacing $\bm{S}_i \to \sum_{l\in\lambda}\bm{S}_{(i,l)}$.
An important example is the projector
\begin{equation}
    P_{i,i+1}^{(J,M)}\wtil{\msf{A}}_{\mr{vb}}=\wtil{\msf{A}}_{\mr{vb}}P^{(J,M)}_{\sum_{l\in\lambda}(i,l),(i+1,l)}\quad ,
\end{equation}
where the projection operator on the right-hand side projects states of the $4S$ spin-$1/2$  from  sites $(i,l)$ and $(i+1,l)$ for $l\in\lambda$ onto the sector with total spin $J$ and $S^z=M$. We write this as $\wtil{P}_{i,i+1}^{(J,M)}$. 

%Like the $S=1$ AKLT case, in addition to the natural choice of the operator $O_{\mr{frac}}$, one can always add to it terms of the form $P_{\sum_{l\in\lambda}(i,l)}^{(J,M)}h_i$ with $J<S$, where $h_i$ is an arbitrary operator. Indeed such operators are annihilated by acting from the left with $\wtil{\msf{A}}_{\mr{vb}}$.
\begin{proof} We define a subspace by restricting the fractional spins with labels $i,R$ and $i+1,L$ to two possible states: a product of singlets, or a fully polarized state. We label these two states as 'up' and 'down' state of a fictitious spin $1/2$. More precisely, we define the map $M_i:\mb{C}^2\rightarrow\mb{C}^{2\otimes 2S}$ for $i\in\Lambda$ as
\begin{equation}\begin{split}
    M_i&\coloneqq\bigotimes_{r\in\{1,\cdots,S\}}\frac{1}{\sqrt{2}}\left(\ket*{\uparrow\downarrow}-\ket*{\downarrow\uparrow}\right)_{(i,r,\mr{R}),(i+1,r,\mr{L})}\bra*{\downarrow}_i+\bigotimes_{r\in\{1,\cdots,S\}}\ket*{\uparrow\uparrow}_{(i,r,\mr{R}),(i+1,r,\mr{L})}\bra*{\uparrow}_i,
    \end{split}
\end{equation}
and $\msf{M}\coloneqq\bigotimes_{i\in\Lambda}M_i$. The image of this map defines the subspace $\mc{W}$ \begin{equation}
    \mc{W}\coloneqq\left\{\msf{M}\ket*{\psi}\big|\ket*{\psi}\in\mb{C}^{2\otimes N}\right\},
\end{equation}
which embeds a fictitious spin $1/2$ chain in the Hilbert space of fractionalized spins.  
We call the projector onto $\mc{W}$ as $P_{\mc{W}}$. In what follows, we write $\ket*{\bm{\sigma}}_{i^*}\coloneqq M_i\ket{\sigma}_i$ with $i^*\coloneqq\sum_{r\in\{1,\cdots,S\}}(i,s,\mr{R}), (i+1,s,\mr{L})$. Note that the VBS state is written as $\ket*{\Phi^{S,\mr{frac}}_{\mr{VBS}}}=\bigotimes_{i\in\Lambda}\ket*{\bm{\downarrow}}_{i^*}$ and the scar states are expressed as 
\begin{equation}\label{eq:scar S-AKLT frac}
    \begin{split}
        &\ket*{\mc{S}^S_n}=\wtil{\msf{A}}_{\mr{vb}}\left(Q_{\mr{frac}}^+\right)^n\bigotimes_{i\in\Lambda}\ket*{\bm{\downarrow}}_{i^*}\eqqcolon\wtil{\msf{A}}_{\mr{vb}}\ket*{\mc{S}_n^{S,\mr{frac}}}\\
        &Q^+_{\mr{frac}}\coloneqq\sum_{i\in\Lambda}(-1)^i\dyad*{\bm{\uparrow}\bm{\uparrow}}{\bm{\downarrow}\bm{\downarrow}}_{i^*,(i+1)^*},
    \end{split}
\end{equation}
up to a normalization factor. It is easy to verify $\ket*{\mc{S}_n^{S,\mr{frac}}}\in\mc{W}$.

As Eq.~\eqref{eq:scar S-AKLT frac} is identical to Eq.~\eqref{SfracAKLT}, a very similar expression of $\ket*{\mc{S}^{S,\mr{frac}}_n}$ to Eq.~\eqref{eq:lemma AKLT} can be found as follows, 
\begin{equation}\label{eq:lemma S-AKLT}\begin{split}
    \ket*{\mc{S}_n^{S,\mr{frac}}}&=\sum_{\bm{\sigma}\bm{\sigma'}}\ket*{\bm{\sigma\downarrow\sigma'}}_{(i-1)^*,i^*,(i+1)^*}\otimes\ket*{\Xi^0_{\sigma\sigma'}}+\left(\ket{\bm{\uparrow\uparrow\downarrow}}-\ket*{\bm{\downarrow\uparrow\uparrow}}\right)_{(i-1)^*,i^*,(i+1)^*}\otimes\ket*{\Xi^1}\\
    &+\ket*{\bm{\uparrow\uparrow\uparrow}}_{(i-1)^*,i^*,(i+1)^*}\otimes\ket*{\Xi^2}\\
    &\equiv\sum_{\bm{\sigma}\bm{\sigma}'}\ket*{\Phi^0_{\bm{\sigma}\bm{\sigma}'}}_{(i-1)^*,i^*,(i+1)^*}\otimes\ket*{\Xi^0_{\sigma\sigma'}}+\ket*{\Phi^1}_{(i-1)^*,i^*,(i+1)^*}\otimes\ket*{\Xi^1}\\&+\ket*{\Phi^2}_{(i-1)^*,i^*,(i+1)^*}\otimes\ket*{\Xi^2},
    \end{split}
\end{equation}
where $\ket*{\Xi^i} (i=0,1,2)$ is an unnormalized state defined on all bonds expect $(i-1)^*, i^*,$ and $(i+1)^*$.

We split $H_{\mr{AKLT}}^S$ into three parts, exactly as the $S=1$ AKLT case,
\begin{equation}\begin{split}
    H_{\mr{AKLT}}^S&=\frac{1}{S}\sum_{i\in\Lambda}S_i^z+\sum_{i\in\Lambda}\left(\sum_{J=S+1}^{2S}\sum_{M=-2S}^{S-1}P_{i,i+1}^{(J,M)}\right)+\sum_{i\in\Lambda}\left(\sum_{J=S+1}^{2S}\sum_{M=S}^{J}P^{(J,M)}_{i,i+1}-\frac{1}{S}S_i^z\right).
    \end{split}
\end{equation}
The first part corresponds to $H_{\mr{spec}}$ and the second part annihilates $\ket*{\mc{S}^S_n}$ as these operators annihilate the ground state ($\ket*{\mc{S}_0^S}$), while excited states ($\ket*{\mc{S}_n^S},\,n>0$) yield a finite result only if they have been acted upon by a spin raising operator with $\Delta M=2S$, starting from a configuration that cannot contain $M=-S-1$ and thus has at least $M\geq -S$. Thus, we should show that the third part also annihilates them. To do so, we fractionalize the third term,
\begin{equation}
    \begin{split}
        &\sum_{i\in\Lambda}\left(\sum_{J=S+1}^{2S}\sum_{M=S}^{J}P^{(J,M)}_{i,i+1}-\frac{1}{S}S_i^z\right)\wtil{\msf{A}}_{\mr{vb}}=\wtil{\msf{A}}_{\mr{vb}}\sum_{i\in\Lambda}T^{\mr{frac}}_{i,i+1}\\
        &T^{\mr{frac}}_{i,i+1}\coloneqq\sum_{J=S+1}^{2S}\sum_{M=S}^J\wtil{P}^{(J,M)}_{i,i+1}-\frac{1}{S}\sum_{r=1}^S\left(S_{(i,r,\mr{R})}^z+S^z_{(i,r,\mr{L})}\right).
    \end{split}
\end{equation}
We shall show that $T_{i,i+1}^{\mr{frac}}$ locally annihilates $\ket*{\mc{S}_n^{S,\mr{frac}}}$ in the sense that $\wtil{\msf{A}}_{\mr{vb}}T_{i,i+1}^{\mr{frac}}\ket*{\mc{S}_n^{S,\mr{frac}}}=0$. From Eq.~\eqref{eq:lemma S-AKLT}, we find
\begin{equation}\label{eq:S AKLT each ann}
    \begin{split}
        &\wtil{P}_{i,i+1}^{(J,M)}\ket*{\Phi^0_{\bm{\sigma}\bm{\sigma}'}}=\frac{1}{S}\sum_{r=1}^S\left(S^z_{(i,r,\mr{R})}+S^z_{(i+1,r,\mr{L})}\right)\ket*{\Phi^0_{\bm{\sigma}\bm{\sigma}'}}=0\,\,(J>S)\\
        &\sum_{J=S}^{2S}\sum_{M=S}^J\wtil{P}_{i,i+1}^{(J,M)}\ket*{\Phi^1}=\frac{1}{S}\sum_{r=1}^S\left(S^z_{(i,r,\mr{R})}+S^z_{(i+1,r,\mr{L})}\right)\ket*{\Phi^1}=\ket*{\Phi^1}\\
        &\sum_{M=S}^{2S}\wtil{P}^{(2S,M)}_{i,i+1}\ket*{\Phi^2}=\frac{1}{S}\sum_{r=1}^S\left(S^z_{(i,r,\mr{R})}+S^z_{(i+1,r,\mr{L})}\right)\ket*{\Phi^2}=\ket*{\Phi^2}.
    \end{split}
\end{equation}
The first line follows from the singlets formed between $(i,r,\mr{R})$ and $(i+1,r,\mr{L})\,\,(r=1\sim S)$ which force the total spin of the sites $i$ and $i+1$ to be at most $S$. The second line follows from the fact that all the local configurations of $\wtil{A}^{\mr{vb}}_i\otimes\wtil{A}^{\mr{vb}}_{i+1}\ket*{\Phi^1}$ have the total magnetization $S_i^z+S^z_{i+1}\geq S$. We then show that $P^{(S,S)}_{i,i+1}$ annihilates $\wtil{A}^{\mr{vb}}_i\otimes\wtil{A}^{\mr{vb}}_{i+1}\ket*{\Phi^1}$. If so, the second line implies $\wtil{A}^{\mr{vb}}_i\otimes\wtil{A}^{\mr{vb}}_{i+1}\sum_{J=S+1}^{2S}\sum_{M=S}^J\wtil{P}_{i,i+1}^{(J,M)}\ket*{\Phi^1}=\wtil{A}^{\mr{vb}}_i\otimes\wtil{A}^{\mr{vb}}_{i+1}\ket*{\Phi^1}$, and then Eq.~\eqref{eq:S AKLT each ann} yields the desired relation $T_{i,i+1}^{\mr{frac}}\ket*{\mc{S}_n^{S,\mr{frac}}}=0$.

To show $\wtil{A}^{\mr{vb}}_i\otimes\wtil{A}^{\mr{vb}}_{i+1}\wtil{P}_{i,i+1}^{(S,S)}\ket*{\Phi^1}=0$, we expand $\ket*{\Phi^1}$ with respect to total magnetization, $\ket*{\Phi^1}=\sum_{M=S}^{2S}c_M\ket*{\Phi^1_M}$ where $c_M$ is a coefficient and $\ket*{\Phi^1_M}$ satisfies
\begin{equation}
    (S_i^z+S_{i+1}^z)\wtil{A}^{\mr{vb}}_i\otimes\wtil{A}^{\mr{vb}}_{i+1}\ket*{\Phi^1_M}=M\wtil{A}^{\mr{vb}}_i\otimes\wtil{A}^{\mr{vb}}_{i+1}\ket*{\Phi^1_M},
\end{equation}
with $M\geq S$. One can find that $\ket*{\Phi^1_S}$ is written as
\begin{equation}\label{eq:|Phi^1_S>}
    \ket*{\Phi^1_S}=\bigotimes_{r=1}^S\ket*{\uparrow}_{(i-1,r,\mr{R})}\left(\ket*{\uparrow\uparrow}_{(i,r)}\ket*{\uparrow\downarrow}_{(i+1,r)}+(-1)^{S+1}\ket*{\uparrow\downarrow}_{(i,r)}\ket*{\uparrow\uparrow}_{(i+1,r)}\right)\ket*{\uparrow}_{(i+2,r,\mr{L})},
\end{equation}
where $\ket*{\sigma\sigma'}_{(i,r)}\coloneqq\ket*{\sigma}_{(i,r,\mr{L})}\ket*{\sigma'}_{(i,r,\mr{R})}$. We then define an operator $sw_{i,i+1}$ acting non-trivially on $\mb{C}^{(2S+1)\otimes 2}$ which implements the site swap of spins at the site $i$ and $i+1$. Eq.~\eqref{eq:|Phi^1_S>} implies that the state $\wtil{A}^{\mr{vb}}_i\otimes\wtil{A}^{\mr{vb}}_{i+1}\ket*{\Phi^1_S}$ is an eigenstate of $sw_{i,i+1}$ with eigenvalue $(-1)^{S+1}$. However, from the general theory of the addition of angular momentum any state in a subspace projected on by $P_{i,i+1}^{(S,M)}\,\,(M=-S\sim S)$ is an eigenstate of $sw_{i,i+1}$ with eigenstate $(-1)^S$, i.e., $P_{i,i+1}^{(S,M)}sw_{i,i+1}=(-1)^SP_{i,i+1}^{(S,M)}$ for $\forall M$. Thus, $\wtil{A}^{\mr{vb}}_i\otimes\wtil{A}^{\mr{vb}}_{i+1}\ket*{\Phi^1_S}$ belong to a different parity sector and is annihilated by $P_{i,i+1}^{(S,S)}$.
\end{proof}

\section{A proof of the Pyramid states}\label{sec:app Pyramid states}
Before giving proof, we introduce $\ket*{\bm{\sigma}_l}$ as a string of $\sigma$'s with length $l$, i.e., $\ket*{\bm{\sigma}_l}=\ket*{\underbrace{\sigma\cdots\sigma}_{l}}$. We also define operators $\sigma_i^{+_l}\coloneqq\dyad*{\bm{\uparrow}_l}{\bm{\downarrow}_l}_{i,\cdots,i+l-1}$ and $\sigma_i^{-_l}\coloneqq\dyad*{\bm{\downarrow}_l}{\bm{\uparrow}_l}_{i,\cdots,i+l-1}$. 

The pyramid state $\ket*{\mc{S}_n^{\mr{Pyr}}}$ is expressed as 
\begin{equation}
    \ket*{\mc{S}_{n,m}^{\mr{Pyr}}}=\sideset{}{'}\sum_{\substack{\{i_k\}_{k=1}^n,\,\{l_j\}_{j=1}^n\\s.t. \sum_jl_j=n+m}}(-1)^{\sum_ki_k}\prod_{q=1}^n\sigma_{i_q}^{+_{l_q}}\bigotimes_{r\in\Lambda}\ket*{\downarrow}_r,
\end{equation}
where $\sum\nolimits'$ means that the sum is over all possible combinations of $\{i_k\}_{k=1}^n$ and $\{l_j\}_{j=1}^n$ with a constraint $i_k+l_k\leq i_{k+1}$.
Thus, the conjugated pyramid states are expressed as
\begin{equation}\label{eq:U|Pyr>}
    U_\pi\ket*{\mc{S}_{n,m}^{\mr{Pyr}}}=\sideset{}{'}\sum_{\substack{\{i_k\}_{k=1}^n,\,\{l_j\}_{j=1}^n\\s.t. \sum_jl_j=n+m}}\prod_{q=1}^n\sigma_{i_q}^{+_{l_q}}\bigotimes_{r\in\Lambda}\ket*{\downarrow}_r.
\end{equation}
The pyramid states can be understood as equal superposition of $n$ domains of upspins with the total length $n+m$. This interpretation allows us to express them in a different way:
\begin{equation}\label{eq:U|Pyr> inverse}
    U_\pi\ket*{\mc{S}_{n,m}^{\mr{Pyr}}}=\sideset{}{'}\sum_{\substack{\{i_k\}_{k=1}^n,\,\{l_j\}_{j=1}^n\\s.t. \sum_jl_j=n+m}}\prod_{q=1}^n\sigma_{i_q}^{-_{l_q}}\bigotimes_{r\in\Lambda}\ket*{\uparrow}_r,
\end{equation}
which is an equal superposition of $n$ domains of $\downarrow$ with the total length $N-n-m$.

This form implies that for any $s<\min\{m,N-2n-m\}$ these states satisfy
\begin{equation}
    \begin{split}
        &P_i^\downarrow P_{i+2}^{\bm{\uparrow}_{s-2}}P_{i+s+2}^\downarrow U_\pi\ket*{\mc{S}_{n,m}^{\mr{Pyr}}}=\sum_{\sigma\sigma'}\ket*{\downarrow\sigma\bm{\uparrow}_{s-2}\sigma'\downarrow}_{i,\cdots,i+s+1}\otimes\ket*{\Xi^\uparrow_{\sigma\sigma'}}\\
        &P_i^\uparrow P_{i+2}^{\bm{\downarrow}_{s-2}}P_{i+s+2}^\uparrow U_\pi\ket*{\mc{S}_{n,m}^{\mr{Pyr}}}=\sum_{\sigma\sigma'}\ket*{\uparrow\sigma\bm{\downarrow}_{s-2}\sigma'\uparrow}_{i,\cdots,i+s+1}\otimes\ket*{\Xi^\downarrow_{\sigma\sigma'}},
    \end{split}
\end{equation}
where $\ket*{\Xi^\tau_{\sigma\sigma'}},\,\,\tau=\uparrow,\downarrow$ is an unnormalized state defined on $\Lambda\setminus\{i,\cdots,i+s+2\}$ and $P_i^{\bm{\sigma}_l}\coloneqq\prod_{k=i}^{i+l-1}P_k^\sigma$. It follows from Eq.~\eqref{eq:U|Pyr>} that $\ket*{\Xi^\uparrow_{\uparrow\downarrow}}=\ket*{\Xi^\uparrow_{\downarrow\uparrow}}$. Thus, $P_i^\downarrow P_{i+2}^{\bm{\uparrow}_{s-2}}P_{i+s+2}^\downarrow U_\pi\ket*{\mc{S}_{n,m}^{\mr{Pyr}}}$ is symmetric under a site swap $i+1\leftrightarrow i+s+1$. Similarly, Eq.~\eqref{eq:U|Pyr> inverse} implies that $\ket*{\Xi^\downarrow_{\uparrow\downarrow}}=\ket*{\Xi^\downarrow_{\downarrow\uparrow}}$, and $P_i^\uparrow P_{i+2}^{\bm{\downarrow}_{s-2}}P_{i+s+2}^\uparrow U_\pi\ket*{\mc{S}_{n,m}^{\mr{Pyr}}}$ is symmetric under a site swap $i+1\leftrightarrow i+s+1$. 

We next show that $H_{\lambda}$ is a sum of \textit{quasi}-local annihilators. In order to define a subspace $\mc{W}$, we define the projector $P_m\coloneqq\prod_{i\in\Lambda}\left(1-\dyad*{\bm{\uparrow}_{m+1}}\right)_{i,\cdots,i+m}$.
The subspace is defined as 
\begin{equation}
    \mc{W}=\left\{\ket*{\psi}\in\mb{C}^{2\otimes N}\big|P_m\ket*{\psi}=\ket*{\psi}\right\}.
\end{equation}
It is easily seen that the Pyramid states belong to this subspace ($\ket*{\mc{S}_{n,m}^{\mr{Pyr}}}\in\mc{W}$) as the length of each domain of upspin cannot exceed $m+2$. $H_\lambda$ is transformed by $U_\pi$ defined in Eq.~\eqref{eq:U DW} as follows,
\begin{equation}\label{eq:UHlamU}\begin{split}
    U_\pi H_\lambda U_\pi^\dag&=2\lambda\sum_{i\in\Lambda}\left(-\dyad*{\downarrow\uparrow\uparrow}{\downarrow\downarrow\uparrow}+\dyad*{\uparrow\uparrow\downarrow}{\uparrow\downarrow\downarrow}\right)_{i-1,i,i+1}\\&+2\lambda\sum_{i\in\Lambda}\left(-\dyad*{\downarrow\downarrow\uparrow}{\downarrow\uparrow\uparrow}+\dyad*{\uparrow\downarrow\downarrow}{\uparrow\uparrow\downarrow}\right)_{i-1,i,i+1}.
    \end{split}
\end{equation}
We now re-write Eq.~\eqref{eq:UHlamU} such that it is a sum of annihilating terms. To do so, we express the identity operator as
\begin{equation}\label{eq:identity string}\begin{split}
    id&=\dyad*{\uparrow}_i+\sum_{k=1}^{N-m-1}\dyad*{\bm{\downarrow}_k\uparrow}_{i,\cdots,i+k+1}+\dyad*{\bm{\downarrow}_{N-m-2}}_{i,\cdots,i+N-m-1}\\
    &=\dyad*{\downarrow}_i+\sum_{k=1}^{N-m-1}\dyad*{\bm{\uparrow}_k\downarrow}_{i,\cdots,i+k+1}+\dyad*{\bm{\uparrow}_{N-m-2}}_{i,\cdots,i+N-m-1},
\end{split}
\end{equation}
where we should use PBC explicitly to identify $i+N=i$ in the strings appears above.

Using Eq.~\eqref{eq:identity string}, Eq.~\eqref{eq:UHlamU} is written as
\begin{equation}
    \begin{split}
        U_\pi H_\lambda U_\pi^\dag P_m&=2\lambda\sum_{i\in\Lambda}\sum_{k=1}^{N-m-1}\ket*{\uparrow\bm{\downarrow}_{k+1}\uparrow}\left(\bra*{\uparrow\uparrow\bm{\downarrow}_k\uparrow}-\bra*{\uparrow\bm{\downarrow}_k\uparrow\uparrow}\right)_{i,\cdots,i+k+1}P_m\\
        &+2\lambda\sum_{i\in\Lambda}\sum_{k=1}^{m+1}\ket*{\downarrow\bm{\uparrow}_{k+1}\downarrow}\left(\bra*{\downarrow\bm{\uparrow}_k\downarrow\downarrow}-\bra*{\downarrow\downarrow\bm{\uparrow}_k\downarrow}\right)_{i,\cdots,i+k+1}P_m\\
        &=2\lambda\sum_{i\in\Lambda}\sum_{k=1}^{N-m-1}P_i^\uparrow P_{i+2}^{\bm{\downarrow}_{k-2}} P_{i+k+1}^\uparrow\ket*{\downarrow\downarrow}\left(\bra*{\uparrow\downarrow}-\bra*{\downarrow\uparrow}\right)_{i+1,i+k}P_m\\
        &+2\lambda\sum_{i\in\Lambda}\sum_{k=1}^{m+1}P_i^\downarrow P_{i+2}^{\bm{\uparrow}_{k-2}} P_{i+k+1}^\downarrow\ket*{\uparrow\uparrow}\left(\bra*{\uparrow\downarrow}-\bra*{\downarrow\uparrow}\right)_{i+1,i+k}P_m.
    \end{split}
\end{equation}
Each term is unaltered when multiplied from the right by a factor $P^{\mr{as}}_{i+1,i+k}P_i^\uparrow P_{i+2}^{\bm{\downarrow}_{k-2}}P_{i+k+1}^\uparrow P_m+(1-P_m)$ or $P^{\mr{as}}_{i+1,i+k}P_i^\downarrow P_{i+2}^{\bm{\uparrow}_{k-2}}P_{i+k+1}^\downarrow P_m+(1-P_m)$ where $P^{\mr{as}}_{i+1,i+k}$ projects onto states antisymmetric with respect to a site swap $i+1\leftrightarrow i+k$. Since the conjugated pyramid states are symmetric when projected by $P_i^\uparrow P_{i+2}^{\bm{\downarrow}_{k-2}}P_{i+k+1}^\uparrow$ or $P_i^\downarrow P_{i+2}^{\bm{\uparrow}_{k-2}}P_{i+k+1}^\downarrow$, these quasi-local operators annihilate them.
